# Supplementary material for: Faster and Better 3D Splatting via Group Training
Source: arXiv:2412.07608 source file (2025-11-24)
Supplement: Supplementary file 1 [file supp.tex]

% ICCV 2025 Paper Template

\documentclass[10pt,twocolumn,letterpaper]{article}

%%%%%%%%% PAPER TYPE  - PLEASE UPDATE FOR FINAL VERSION
\usepackage{iccv}              % To produce the CAMERA-READY version
% \usepackage[review]{iccv}      % To produce the REVIEW version
% \usepackage[pagenumbers]{iccv} % To force page numbers, e.g. for an arXiv version

% Import additional packages in the preamble file, before hyperref
\input{preamble}
%%%%%%%%%%%%%%%% CUSTOM PACKAGES %%%%%%%%%%%%%%%%
\usepackage[table]{colortbl}
\usepackage{multirow}
% \usepackage{enumitem}
% \usepackage{arydshln}
% \usepackage{verbatim}
% \usepackage{setspace}
% \usepackage{nicefrac}
% \usepackage{graphicx}
%%%%%%%%%%%%%%%% CUSTOM PACKAGES %%%%%%%%%%%%%%%%

% It is strongly recommended to use hyperref, especially for the review version.
% hyperref with option pagebackref eases the reviewers' job.
% Please disable hyperref *only* if you encounter grave issues, 
% e.g. with the file validation for the camera-ready version.
%
% If you comment hyperref and then uncomment it, you should delete *.aux before re-running LaTeX.
% (Or just hit 'q' on the first LaTeX run, let it finish, and you should be clear).
\definecolor{iccvblue}{rgb}{0.21,0.49,0.74}
\usepackage[pagebackref,breaklinks,colorlinks,allcolors=iccvblue]{hyperref}

%%%%%%%%% PAPER ID  - PLEASE UPDATE
 % *** Enter the Paper ID here

%%%%%%%%% TITLE - PLEASE UPDATE
\title{Faster and Better 3D Splatting via Group Training}

%%%%%%%%% AUTHORS - PLEASE UPDATE
\author{
Chengbo Wang\textsuperscript{1,2} \qquad
Guozheng Ma\textsuperscript{3} \qquad
Yifei Xue\textsuperscript{1,2,4,5} \qquad
Yizhen Lao\textsuperscript{1,4,5,$\dagger$} \\
\textsuperscript{1}Hunan University \quad \textsuperscript{2}DaHe.AI \quad \textsuperscript{3}Nanyang Technological University  \quad
\textsuperscript{4}Lushan Lab 
\\
\textsuperscript{5}The Key Laboratory of Ministry of Culture and Tourism, 
\\ Intelligent Design Technology for Digital Cultural Creativity Lab
\\
{\tt\small \{wangchb, yizhenlao\}@hnu.edu.cn, GUOZHENG001@e.ntu.edu.sg, iflyhsueh@gmail.com}
}

\begin{document}

\input{sec/X_suppl}

{
    \small
    \bibliographystyle{ieeenat_fullname}
    \bibliography{main}
}

\end{document}
